# Supplementary material for: Ultrafast switching to a stable hidden topologically protected quantum state in an electronic crystal
Source: arXiv:1401.6786 source file (2014-04-07)
Supplement: Supplementary file 1 [file 1241591Supplementary_material.pdf]

# Supplementary Materials for Ultrafast switching to a stable hidden topologically protected quantum state in an electronic crystal


L. Stojchevska[1,2], I. Vaskivsky[1], T. Mertelj[1], P. Kusar[1],

D. Svetin[1], S.Brazovskii[4,5] and D. Mihailovic[1,2,3*]

[1]*Dept. of Complex Matter, Jozef Stefan Institute, Jamova 39, Ljubljana, SI-1000, Ljubljana, Slovenia*

[2]*Jozef Stefan International Postgraduate School, Jamova 39, Ljubljana, SI-1000, Ljubljana, Slovenia*

[3]*CENN Nanocenter, Jamova 39, Ljubljana, Slovenia*

[4]*LPTMS-CNRS, UMR8626, Univ. Paris-Sud, Bat. 100, Orsay, F-91405, France and*

[5]*International Institute of Physics, 59078-400 Natal, Rio Grande do Norte, Brazil*



*Electronic address: dragan.mihailovic@ijs.si

Contents

I. Sample details 2

II. Experimental details 3

III. Calculation of the electronic and lattice temperatures after a Write (W) pulse 4

IV. Calculation of the temperature after the Erase (E) pulse burst. 6

V. The calculation of the system trajectory 8

VI. Bimodal switching and power dependence in stroboscopic experiments 14

VII. Comparison of mode frequencies observed by Raman and coherent phonon spectroscopy in different phases of $TaS_2$. 14

References 17

## I. SAMPLE DETAILS

Numerous samples of two different origins were used to check for consistency of the results. Fresh *1T*-$TaS_2$ samples were grown by P. Sutar and A. Mrzel by first synthesizing $TaS_2$ powder from the elements (99.9% Ta foil, 99.98% S powder) in a stoichiometric ratio (with 99.98% iodine as transport agent) in a quartz ampoule and heated in a multiple zone furnace 750 °C - 850 °C for 5 days. The ampoule was subsequently opened and resealed with a small quantity of $C_{60}$ powder as getter, then heated in a multiple-zone furnace with a temperature gradient of 900 °C - 800 °C for 6 hours, subsequently reversing the gradient to 750 °C - 850 °C for 8 days. Finally, the ampoule was quenched into water. The single crystals, up to 5×5×0.1 mm in size were checked by Raman, resistivity and XRD to be the *1T*-$TaS_2$ polytype. *1T*-$TaS_2$ samples from G. Berger were grown at EPFL as described in [1]. They were already used for measurements in 2002 [2, 3]. No significant difference was observed in the data from the two sets of samples.

## II. EXPERIMENTAL DETAILS

The samples were mounted on a cold finger of a liquid-He flow optical cryostat equipped by $CaF_2$ windows.

For the optical measurements, all the laser beams were derived from a 250-kHz-repetition-rate regenerative Ti:$Al_2O_3$ laser amplifier with 50 fs pulse length. Acousto-optic modulators (AOM) were used to modulate the beams. The modulators for W and E beam were controlled by a programmable function generator synchronized to the laser in order to pick a desired number of pulses from the original pulse train. The modulator for the pump (P) beam was controlled by a lock-in amplifier using a a standard 2-pulse pump-probe detection scheme.

The W-pulse length was increased from the original length of 50 fs either by increasing the accumulated dispersion in the amplifier by varying the number of the amplifier round trips or adjustments of the post-amplification optical pulse compressor, that was used also to compensate the dispersion of the AOMs. The E pulses of ~50 ps length were derived from the uncompressed amplifier output by bypassing the compressor.

For the resistance measurements, a single pulse from an amplified Ti:Sapphire laser (Coherent Legend) was used with a 35 fs pulse length. The sample was illuminated from the back side through the sapphire substrate to achieve uniform illumination and to ensure that there is no unilluminated gap between the contacts and the sample.

The resistance $r(T)$ was measured by the standard 4-contact technique. Gold contacts $\sim$ 10 $\mu$m apart were manufactured by laser lithography using a LPKF ProtoLaser LDI machine, which allows lithography on samples deposited on an insulating substrates using a 2-layer photoresist (Allresist ARP 5480/ARP3510). The samples used in the experiments were 80-100 nm thick exfoliated *1T*-$TaS_2$ single crystals which were previously deposited on a sapphire substrate by exfoliation from sticky tape. (The temperature dependence of the resistivity for thinner samples is no longer characteristic of *1T*-$TaS_2$, from which we conclude that the strain caused by the contraction mismatch between the substrate and the sample modifies the system to such an extent that we are no longer dealing with characteristic *1T*-$TaS_2$ material.) The I-V characteristics were measured at each temperature, and were linear in a range $\pm$100 $\mu$A. Erasure by Joule heating was achieved by passing a current of 1 mA.

*1T*-$TaS_2$ is known to have slow relaxation dynamics associated with pinning and/or

intersecting discommensurations which can strongly affect the measurements unless a proper protocol for thermal cycling is followed [4, 5]. We have used a thermal cycling protocol which gave us consistent results: **all** cooling cycles were done starting at room temperature, and temperature was changed at a rate of 2 K/minute or slower. Once switched, thermal annealing was done by heating to room temperature. Interrupting the thermal cycle at intermediate temperatures gave unpredictable results.

Importantly, the threshold measurements were done by measurement of the AM switching. This means that the same volume is switched and probed, as determined by the optical penetration depth, which is equal for both the W excitation and the probe. For the resistivity measurements, we need to illuminate from the back, because illuminating from the front creates shadows. However, since the thickness is greater than the penetration depth, we need to use higher fluences with back illumination, to ensure that the contact region is illuminated above threshold. Typically this is found to be 3-4 times the the threshold fluence as determined from optical measurements. The entire sample is thus exposed to above-threshold excitation, which gives us the reproducible resistance switching characteristics.

## III. CALCULATION OF THE ELECTRONIC AND LATTICE TEMPERATURES AFTER A WRITE (W) PULSE

The temperature after photoexcitation can be estimated using Newton's law of cooling, with the electrons and the lattice assumed to be described by effective temperatures $T_e$ and $T_L$ respectively:

$$\gamma_e T_e \frac{dT_e}{dt} = -\gamma_L (T_e - T_L) + P(t), \tag{1}$$

$$C_L(T) \frac{dT_L}{dt} = \gamma_L (T_e - T_L), \tag{2}$$

By meticulously taking into account the $T$-dependent specific heats $\gamma_e(T)$ and $C_L(T)$, the optical absorption coefficient $\alpha$ and reflectivity $R$ of *1T*-$TaS_2$ at 800 nm, the uncertainty of the calculated $T_e$ and $T_L$ can be significantly reduced. $P(t) = (1-R)\frac{E_0}{\sqrt{2\pi}w} exp\left[-\frac{(t-t_0)^2}{2w^2}\right]$ is the normalized W pulse intensity, where $\tau_W = 2\sqrt{2\ln 2}w$ is the W pulse width. $\gamma_L = 3\hbar\lambda_{e-p}\langle\omega^2\rangle\gamma_e/\pi k_B \simeq 300\text{psK}^{-1}$ is the energy relaxation rate [6], and $\gamma_e = 4.2$ mJmol$^{-1}$K$^{-2}$

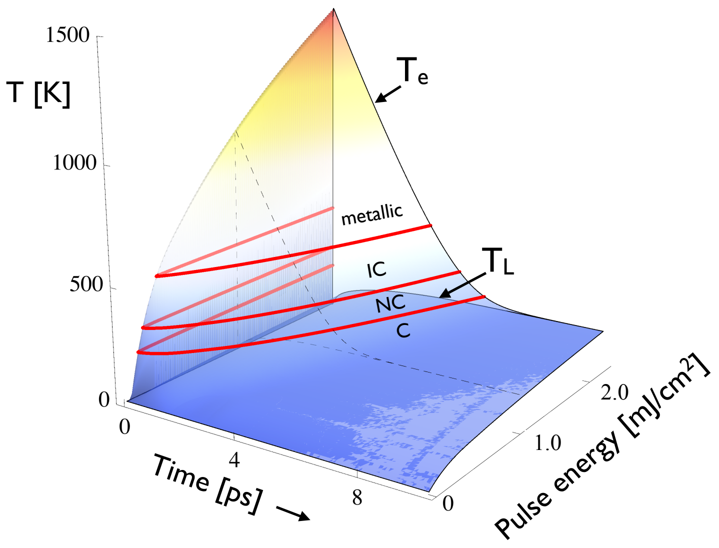


FIG. S1: The estimated temperatures $T_e$ and $T_L$ after excitation calculated using the 2TM as a function of pulse energy $U_W$. The dashed line represents the threshold value of $U_W$ for the transition to the $H$ state. The red lines indicate the transition temperatures $T_{c0}, T_{c1}$ and $T_{c2}$ respectively.

is the electronic specific heat coefficient[7]. $C_L(T)$ is the lattice specific heat and $R = 0.6$ is the reflectivity at 800 nm[8]. Using an electron-phonon interaction constant $\lambda_{e-p} \sim 0.25$, a Debye model fit of the experimental $C_L(t)$ [9] and an estimated second moment of the Debye frequency $\langle \omega^2 \rangle \sim 10$ THz$^2$, we obtain the evolution of $T_e(t)$ and $T_L(t)$ as a function of $E_0$ and $\tau_W$ shown in Fig. S1. At the threshold for switching, the calculated $T_L$ is ∼150 K. $T_e$ initially reaches 1400 K, but becomes comparable to the lattice temperature on a timescale of ∼ 3 ps.

To test the accuracy of the calculation, we compare the calculated $T_L$ to the measured temperature of the lattice obtained from the time dependence of the amplitude mode frequency $\omega_{AM}$ measured using the 3-pulse technique [20], and its independently determined temperature-dependence. We see that the calculated and measured $T_L$ agree to better than 10 K (Fig. S2).

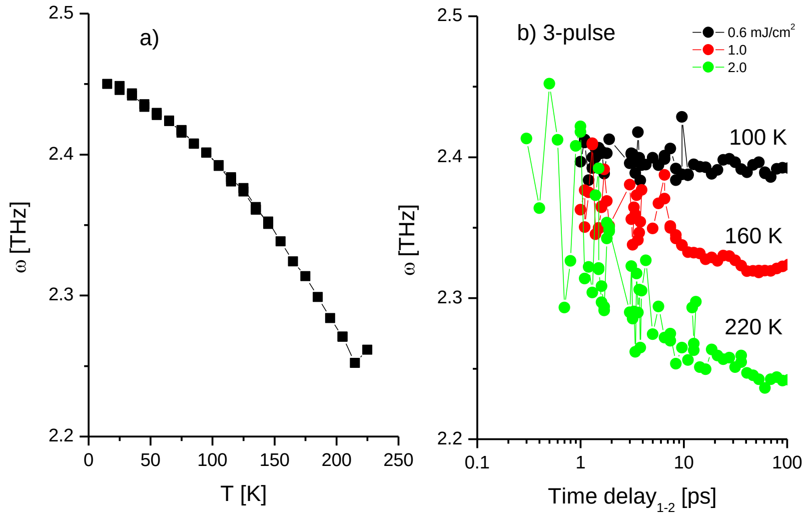


FIG. S2: a) The measured frequency of the AM as a function of temperature using the Pump-probe technique (see also ref. [2]). b) The frequency of the AM as a function of time after a W pulse of different magnitude measured as a function of time delay by the Pump-probe method. The three curves correspond to $U_W = 0.6$, 1.0 and 2.0 mJ/cm$^2$, using 50 fs pulses shown by black, red and green data points respectively. The lattice temperature reached after 100 ps for the three pulse energies are approximately 100 K, 160 K and 205 K respectively. The middle curve corresponds to the threshold value of $U_w$. The measured temperatures are in remarkable agreement with the calculated ones on the basis of the two temperature model shown in Fig. S1. Note that the large oscillations at early times are not noise, but rather they are order parameter oscillations which occur at early times[20].

## IV. CALCULATION OF THE TEMPERATURE AFTER THE ERASE (E) PULSE BURST.

The average surface temperature between the transient $T$ spikes during a long burst of pulses can be approximated by solving a steady state anisotropic heat conduction model [10]. We need to take into account the strong $T$-dependence of the heat conductivity [11] below $T_{c2}$. Furthermore, an absence of experimental data on the out-of-plane heat conductivity means that the diffusive heat transport perpendicular to the surface can only be qualitatively estimated. Using the average power density for the the case of erase pulses, the in-plane heat

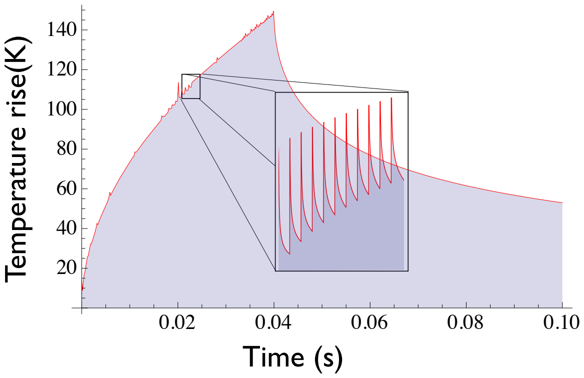


FIG. S3: The calculated lattice temperature rise $\Delta T_L$ as a result of the $E$ burst, a pulse train of $10^4$ pulses, each $\tau = 50$ ps in length and 4 $\mu$s apart. The constants are $K_c = 0.01$ W/cm-K, $\rho = 6$ g/cm$^3$. The value of $K_c$ is an estimate from the measured in-plane thermal conductivity of $K_{ab} = 0.1$ W/cm-K [11]. The uncertainty in estimated temperature comes mainly from the uncertainty in thermal conductivity perpendicular to the sample surface.

conductivity at 100 K, $K_{\rm par} \simeq 0.1$ W/cmK,[11] and assuming, that the out-of-plane heat conductivity, $K_{\rm perp}$, is 10-100 times smaller than $K_{\rm par}$, we obtain the surface temperature rise in the 40-120 K range.

Let us next estimate the time for the temperature to drop below $T_H$ after absorption of a single pulse. Initially the energy is absorbed within the optical penetration depth, $\lambda_{\rm opt} \simeq 20$ nm, thick layer [8]. Since the beam diameter, $w_{FWHM} = 86$ $\mu$m, is much larger than $\lambda_{\rm opt}$ the diffusion is effectively 1D. The characteristic diffusion length is estimated from the ratio of the internal energies, $\xi \simeq \lambda_{\rm opt} U(T_0)/U(T_{\rm c}')$, obtained by extrapolating the heat capacity data[9] using Debye model, where $T_0$ is the initial temperature immediately after the system thermalizes. Assuming the same anisotropy as above we estimate the thermal diffusivity, $\kappa_{perp}$, to be in the $\sim 2 \cdot 10^{-4} - 4 \cdot 10^{-3}$ cm/s$^2$ range between $T_p$ and room temperature, resulting in the characteristic time for diffusion $\tau_{\rm SP} = \xi^2/4\kappa_{perp}$ in the $\sim 2 - 300$ ns range. Here the longest $\tau_{\rm SP}$ corresponds to the smallest $\kappa_{perp}$ and $T_0 \simeq 300$ K corresponding to

the case of erase pulse. In the case of the write pulse at the threshold $T_0 \sim 200$ K, giving $\tau_{SP} < 30$ ns.

Bearing this in mind, the surface temperature rise resulting from the E pulse burst is calculated using a solution to the diffusion equation with appropriate boundary conditions[10]. Simplifying the pulse shape to a square hat top, the surface temperature rise from the accumulated heat, expressed as a summation over the whole pulse train of $N$ pulses is given by:

$$\Delta T_L = \frac{2U_E(1-R)}{\tau_W K}\sqrt{\frac{\kappa\tau}{\pi}}\sum_{n=0}^{N}\Theta[(x-t_0-\tau)]Re\left[\sqrt{\frac{x-nt_0}{\tau}}-\sqrt{\frac{x-nt_0}{\tau}-1}\right] \qquad (3)$$

where $\Theta$ is the heaviside theta function, $t_0$ is the time between pulses, $\tau$ is the individual pulse duration, $R$ is the reflectivity, $K$ is the thermal conductivity, $\kappa = {}^{K}\!/_{\rho c}$ is the thermal diffusivity, $c$ is the specific heat capacity and $\rho$ is the density of *1T*-$TaS_2$ [7]. The temperature dependence of $K$ arising from the thermal conductivity and specific heat are explicitly taken into account, just as in the W pulse calculation. The estimated $\Delta T(t)$ is plotted in Fig. S3.

## V. THE CALCULATION OF THE SYSTEM TRAJECTORY

We present a plausible phenomenological theory with the aim of elucidating the underlying physics. The main requirements are that (1) it should be as simple as the problem allows, (2) it is still computationally treatable, which is not trivial considering the highly non-linear nature of the phenomenon which it needs to describe, (3) it needs to be compatible with the existing microscopic picture of this material and (4) it needs to describe the three main remarkable observations of the experiment. The proposed model is independent of underlying microscopic details and can be elaborated and extended further, but the minimal model which we give here satisfies the requirements above and the numerical solutions of the equations presented below are successful in describing the system trajectories for the different cycles performed in the experiments.

We need a mechanism by which a new ordered state forms under nonequilibrium conditions, rather than the system simply returning to the ground state.The important fundamental insight of the model is the necessity for a transient electron-hole asymmetry at the Fermi level, which allows a transient photodoping effect to occur just long enough for a new

hidden state to form. The energy relaxation timescale for photoexcited carriers where the asymmetry originates also relates to the switching timescale observed in our experiments. Once the state is established, its collective nature protects it from dissipating.

The focus of the model is on three reservoirs of electrons: electrons and holes as mobile charge carriers with concentrations $n_e$ and $n_h$ and the crystallized electrons with the concentration $1 - n_d$ where $n_d = n_v - n_i$ is the relative density of intrinsic defects (interstitials "i" and voids "v" as explained in the main text; both of which are known to be present [12]). All together, the concentrations are subject to the charge conservation law $n_e - n_h = n_v - n_i = n_d$.

The total free energy, which we shall consider additive, $F(n_d, n_e, n_h) \approx F_d(n_d) + F(n_e) + F(n_h)$ determines the partial chemical potentials (in photo-physics of semiconductors they are also referred to as quasi-Fermi levels) $\mu_j = \partial F / \partial n_j \approx \mu_j(n_j)$ (these are also functions of the temperature) of the reservoirs which must be all equilibrated in the final static regime. The electrons and the holes from the nominally empty and filled band states will be considered as particles with 2D spectra $\epsilon_{e,h}(p) = \Delta_{e,h} + p^2/2m_{e,h}$ characterized by their activation energies - the gaps $\Delta_{e,h}$ and by effective masses $m_{e,h}$ giving constant densities of states $N_{e,h} \sim m_{e,h}$ above the respective gaps. That yields the chemical potentials as

$$\mu_{e,h}(n) = \Delta_{e,h} + k_B T \ln(e^{n_{e,h}/(k_B T N_{e,h})} - 1). \tag{4}$$

The necessary free energy $F_d(n_d)$ of the crystalline reservoir can be taken just to satisfy the fact of the first order phase transition in equilibrium between the $C$ and $IC$ phases, which is the experimental fact as well as the results of thermodynamical calculations. We went a bit further to justify the chosen form of $F_d$ by referring to a general theory [13] of weakly incommensurate triangular lattices. Assuming the symmetry between vacancies and interstitials, i.e. with respect to the sign of $n_d$, we choose the parametrization

$$F_d(n_d) = E_{DW}(C_0|n_d| + C_1|n_d|e^{-1/(\xi|n_d|)} - C_2\xi n_d^2 + C_4\xi^3 n_d^4) \tag{5}$$

where $C_n$ are numeric constants. Here $\xi$ is the domain wall width and $E_{DW}$ is its energy scale per constituent defect. The first two terms are standard for a picture of the $C$-$IC$ transition [13]: in thermodynamic equilibrium, the coefficient $C_0 < 1$, as a function of $T$, reduces the DW energy and for $C_0 < 0$ the walls start to be created but their concentration

is stabilized by the repulsion given by the second term $\sim C_1$. The next term $\sim C_2$ appears for non-collinear arrays of domain walls which now intersect in points with a concentration $\sim n_d^2$. A key point [13] is that this energy is expected to be negative, which we took into account with the sign "-" of the term $\sim C_2$ in (5). Together with the last stabilizing term $\sim C_4$ to take into account the repulsion between the crossings, we obtain the desired non-monotonous curve for $F_d$ shown in Fig. 3 B of the main text. The chemical potential of the crystalline reservoir is then:

$$\mu_d(n_d) = E_{DW}(C_0 + C_1(1 + \frac{1}{\xi|n_d|})e^{-1/(\xi|n_d|)} - 2C_2\xi|n_d| + 4C_4(\xi|n_d|)^3)\text{sign}(n_d). \qquad (6)$$

The three surfaces of chemical potentials $-\mu_e$, $\mu_h$ and $\mu_d$ as a function of $n_e$, $n_h$ with $n_d = n_e - n_h$ respectively are shown in Fig. 3 D of the main text. ($\mu_h$ and $\mu_d$, as both counting the electron's deficiencies, should be always taken with an opposite sign with respect to $\mu_e$.)

Recent experiments show that the Mott gap rapidly melts within $\sim$ 50 fs after photo-excitation [14], but after 0.5 $\sim$ 1 ps, the AM oscillations are visible again, indicating the recovery of the CDW state within a few AM cycles. Since the *e-h* energy relaxation occurs on a similar timescale ($\tau_E \sim$ 1 ps) [2, 14], the condensation into the crystalline state competes with $e - h$ recombination.

Mutual transformations among the reservoirs, together with the concommitant heat production, are dictated by imbalances of the three partial chemical potentials $\mu_j$. To model the nonequilibrium evolution, we need to consider the relaxation kinetics between the three reservoirs. The corresponding kinetic equations are chosen to have the simplest form which satisfies the condition that the exchange rate among any two reservoirs vanishes when the corresponding chemical potentials become equal $\delta\mu_{i,j} = 0$. A schematic diagram of the relaxation processes is shown in Fig. 3C of the main text.

The rates $R_{ij}$ of particles' exchange among the reservoirs may be complicated functions of $n_j$, $\mu_j$, and $T$ and we need to make physically motivated model assumptions. It is common in the physics of semiconductors, as well as gapped correlated electron systems, to take the bi-particle form for the $e - h$ recombination $R_{eh} \sim n_e n_h$ [18, 19]. Linear terms $R_{hd} \sim n_h$ and $R_{ed} \sim n_e$ imply that the band particles can transform into defects without meeting another particle, e.g. holes can annihilate with polarons neglecting the small concentration of defects. In principle the bi-modal parts $R_{ed}^{bm} \sim n_e n_d$ and $R_{hd}^{bm} \sim n_e n_d$ can be also present,

but we will neglect such higher order terms to keep the model simple. Next we use the most general principle that, when the potentials are mismatched, $R_{ij}$ changes sign, passing through zero when the potentials coincide: $\delta\mu_{i,j} = 0$. Again, we use the simplest form of the linear dependence $R_{ij} \sim \delta\mu_{i,j}$. Finally, kinetic equations for the time evolution of $n_h(t)$ and $n_e(t)$ acquire the form:

$$\frac{dn_h}{dt} = -k_{eh}n_e n_h(\mu_e + \mu_h) - k_{hd}n_h(\mu_h - \mu_d) \; + P(t) \tag{7}$$

$$\frac{dn_e}{dt} = -k_{eh}n_e n_h(\mu_e + \mu_h) - k_{ed}n_e(\mu_e + \mu_d) \; + P(t) \tag{8}$$

where $k_{ij}$ are the coefficients of the recombination rates $R_{i,j}$ after extracting dependencies on $n_{i,j}$ and $\delta\mu_{i,j}$, $P(t)$ is the temporal profile of particles production. As a further justification of the equations above, notice a distant resemblance of these equations with the basic equations describing photo-voltaic devices (see e.g. [18, 19]); superficially, $n_d$ can be compared with electrons trapped by impurities or lattice defects.

The temperature evolution during the cycle is taken into account by the energy balance equation

$$J = C_T dT/dt = \sum_j \mu_j (dn_j/dt), \tag{9}$$

where $C_T$ is the effective heat capacity of the electronic system. To keep the model as simple as possible, we consider here the part of the cycle which is relevant for establishing the ordered state. (The subsequent cooling of the electronic system to the lattice can be treated separately by lowering the temperature externally to the model, by introducing additional lattice bath into the system of equations via the two-temperature model (Eqs. (1) and (2)), or even extending it to take into account thermal diffusion processes; later we discuss the inclusion of the two-temperature model). The formulas (7,8) and (9) form a complete set of equations governing the system evolution on transition to a charge ordered state under photodoping conditions. Their solution yields the trajectories shown in Fig. 4 of the main text. The time dependencies of $n_e$, $n_h$ and $n_d$ are shown in Fig. S4.

In these calculations, the time is in ps (defined by the rate constants $k_{ij}$ which are in ps$^{-1}$), the laser pulse length is taken as $\tau = 0.035$ ps. Other quantities are dimensionless: $n_j$ as concentrations per enlarged unit cell of one star; the energies as given in units of the electrons' gap $\Delta_e$. The parameters used for calculation presented in the main text and in

Fig. S4 below are as follows. The hole gap is taken as $\Delta_h = 1.4$ (following a prevailing experimental information and band calculations that the Fermi level is closer to the upper band edge). The densities of states are $N_h = 1.2$, $N_e = 1$ (from indications on the bandwidths in the literature). For electrons there may be an uncertainty because we do not know for sure if they thermalize to the bottom of the conduction band or to the upper Hubbard level whose positions are close to each other, see [15] and refs. therein. Also the electronic states are not accessible to photo-emission experiments. But still, it is known from STS [16] and optics [17] that the total gap is $\Delta_e + \Delta_h = 0.6eV$, so our energy unit is 0.25eV.

Parameters in Eqs. (5,6) are adjusted such that the free energy $F_d$ shows the appropriate minimum as plotted in Fig. 3 B of the main text: $C_0 = 0.22$, $C_1 = 1$, $C_2 = 1$ and $C_4 = 2$. The domain wall size is $\xi = 3$, in lattice units, and the domain wall energy scale is $E_{DW} = 2$. So the energy to initiate one defect is taken as $E_d = C_0 E_{DW} = 0.44\Delta_e = 0.11eV$. $k_{eh} = 20$ ps$^{-1}$ , $k_{hd} = 20$ ps$^{-1}$ and $k_{ed}$ =10 ps$^{-1}$; their magnitudes are estimated from the observed single particle relaxation rate in Fig. 2 B of the main text. The trajectory is very robust with respect to parameters $k_{ij}$, changing their magnitude by a factor of 2 has a minor effect on the solutions, provided that the asymmetry $k_{hd}/k_{ed} > 2$. For these parameters, the threshold laser pulse energy for switching to the $H$ state is $U_T = 0.8$.

The temporal evolution of $n_e$, $n_h$, $n_d$ and $T$ is plotted in Fig. S4 above and below $U_T$, corresponding to the trajectories shown in Fig. 4 A and B of the main text. Notice that the temperature saturates quite fast while the evolution of concentrations requires a much longer time to reach the H state (Fig. S4 A), and an even longer time towards the C state (Fig. S4 B).

The cooling part of the cycle has so far not been addressed in the model. In principle, we need to discuss the energy relaxation to the lattice bath, (such as in the two-temperature model described in Sec. III) and the eventual thermal diffusion out of the photo excited volume. Including the two-temperature model in the relaxation process (Eqs. (1) and (2)) requires solving them together with Eqs. (7) and (8). In Fig. S4 C we show the calculation of $n_e$, $n_h$, $n_d$, as well as the electronic and lattice temperatures $T_e$ and $T_L$, respectively for such a model. We observe that for $n_e$, $n_h$, $n_d$ qualitatively similar behaviour is seen as in the minimal model.

The stability of the final H state in the final stage of relaxation is protected by the form of the free energy (5), which ensures the stability of a charge ordered state with $n_d \neq 0$ and $\delta q \neq$

0. Recovery to the ground state ($n_d = 0$ and $\delta q = 0$) involves the introduction or removal of additional periods in the electronic crystal order, which is energetically costly, and is thus inhibited as discussed in the main text. Further discussion of the system evolution in this regime, and associated thermal relaxation is beyond the scope of the present experimental data set.

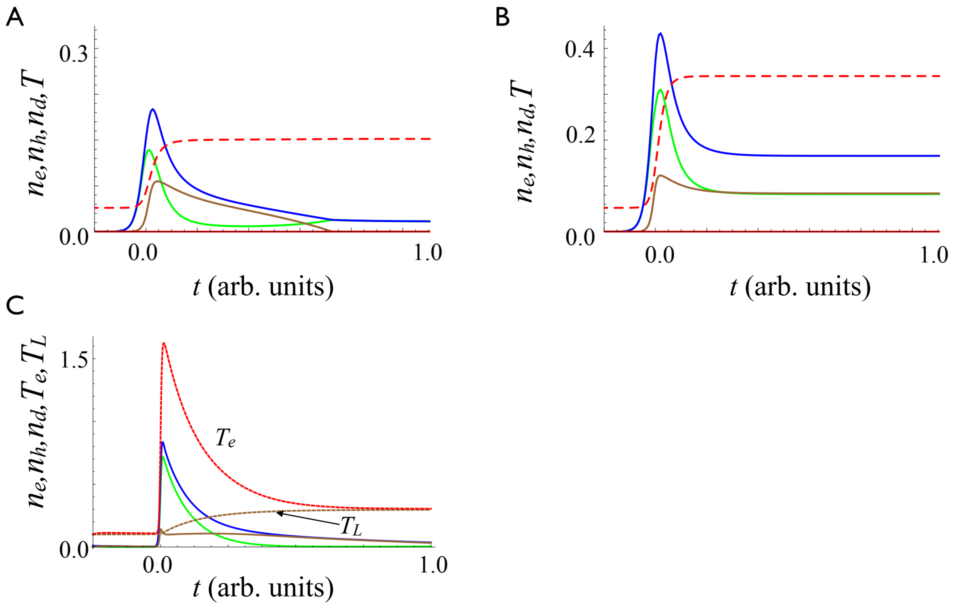


FIG. S4: The calculated $n_e$ (blue), $n_h$ (green), $n_d$ (brown) and the temperature $T$ (red dashed) as functions of time using the equations (7,8) and (9): a) below threshold ($U_W < U_T$) and b) above threshold ($U_W > U_T$). The initial temperature was taken as $T = 0.1\Delta_e/k_B$. The corresponding parametric plots of $n_e$ and $n_h$ are shown in Figs. 3 D and E respectively of the main text. Note that the calculation does not discuss the cooling part of the cycle, so the temperature remains high after all the pulse energy is transferred. In C we show the results of a calculation which includes the two-temperature model (Eqs. (1) and (2)) for $U_W > U_T$. $n_e$ (blue), $n_h$ (green), $n_d$ (brown) are qualitatively similar to the results of the simple model calculation (B). The electronic and lattice temperatures $T_e$ and $T_L$ are shown by the red-dashed and brown-dashed lines respectively.

## VI. BIMODAL SWITCHING AND POWER DEPENDENCE IN STROBOSCOPIC EXPERIMENTS

Additional insight into the switching mechanism may be obtained from measurements of the dependence of the collective mode spectrum on the laser pulse fluence $U_W$, particularly near threshold fluences. In Fig. S5 A and B we first show the transient reflectivity and the resulting FT spectra measured by increasing the power of the pump pulse with the standard Pump-probe technique. The spectra do not show any clear switching behaviour. Instead, the spectrum broadens and some spectral weight shifts towards lower frequency. Upon reducing the pump power, the spectrum measured thereafter with low power reverts to the H state spectrum, as shown in Fig. 2 B of the main text. For comparison, we also show the reflectivity transients *after exposure to single W pulses with different fluences*, measured with standard (low-power) Pump-probe spectroscopy. We observe a clear bimodal distribution for the AM with two modes at 2.39 and $\sim$ 2.45 THz, and no spectral density in between. The higher frequency modes are also shown. The threshold behaviour is quite pronounced.

## VII. COMPARISON OF MODE FREQUENCIES OBSERVED BY RAMAN AND COHERENT PHONON SPECTROSCOPY IN DIFFERENT PHASES OF TAS$_2$.

To show that a light-induced structural transition to a known thermodynamic phase is not taking place, we can compare the spectra of the H state (shown in Fig.2 of the main text) with Raman spectra of all know phases and polytypes of $TaS_2$ at different temperatures listed in Table 1. From the absence of any correspondence between the published fingerprint spectra and the measured H state spectrum we conclude that structural switching to any known thermodynamic phase does not take place. Note that the IR modes should not be observable in our coherent phonon spectra, where only Raman-active modes are allowed.

Further, to demonstrate that the H state spectrum is different from the NC state (on cooling) or the T state (on warming), we show the spectra measured by coherent phonon spectroscopy with the Pump-probe technique in Fig. S6. Two major things are different between the NC and the H state: (1) there is no exponential background in the NC state, which is quite pronounced in the H state and (2) the spectrum of the NC state is quite

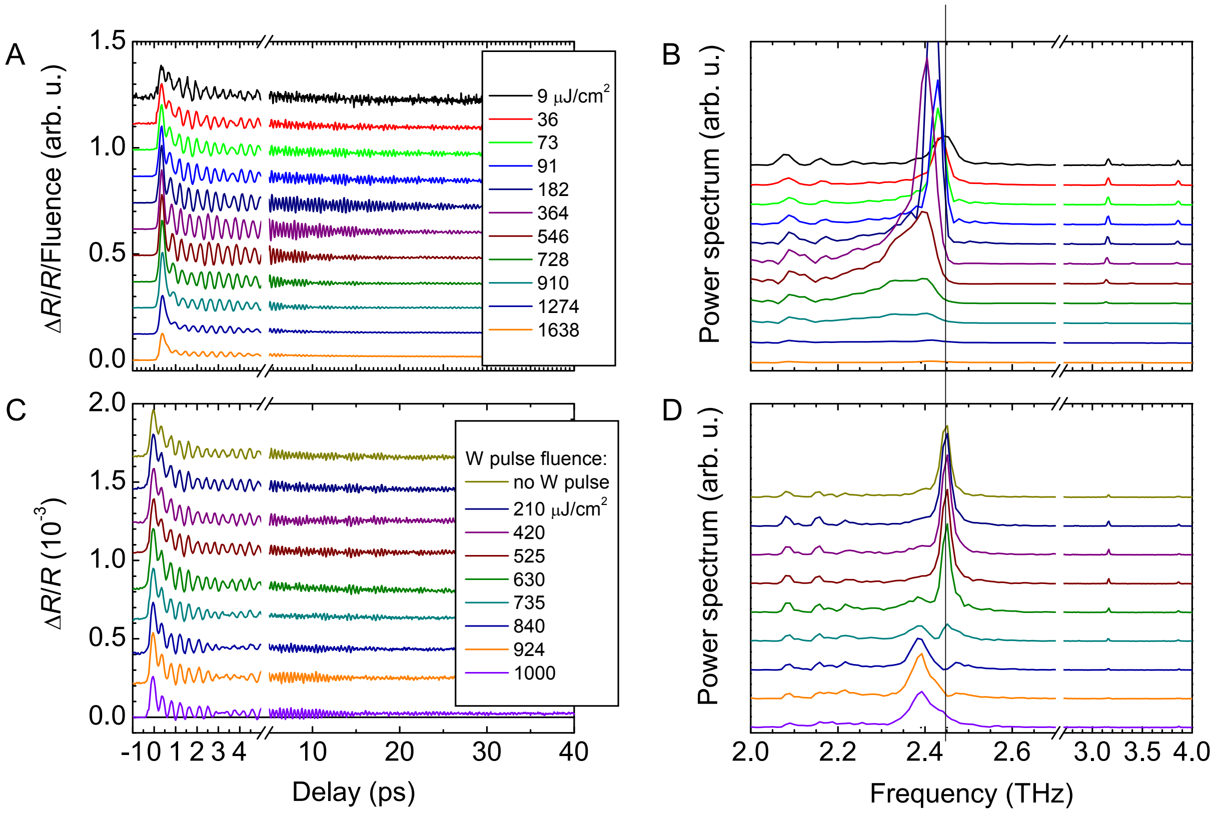


FIG. S5: A. Transient reflectivity traces at different pump power measured by a stroboscopic pump-probe experiment at a 250kHz repetition rate. B. The corresponding power spectra show a broadening and a shift to lower frequency with increasing pump power. The data are normalised to pump power. C. The reflectivity traces in three-pulse measurements: The fluence of the (single) W pulse is varied, but the measurements are made with a pump-probe sequence with very low pump and probe power. D. The corresponding power spectra show bimodal switching behaviour between 2.39 and 2.46 THz. For W near threshold two distinct modes are abserved, but no spectral density in between. All the data were obtained with 50 fs pulses at 800 nm.

different. It is weak, and exhibits a relatively broad spectral feature centred around 2.1 THz. The NC and T states are thus quite different from the H state, which - at least regarding the mode spectra - is more similar to the C state than either of the high-temperature states.

| *1T*-$TaS_2$* | *H*-$TaS_2$ | *1T*-$TaS_2$ | *1T*-$TaS_2$ | *1T*-$TaS_2$ | *2H*-$TaS_2$ | *4Hb*-$TaS_2$ | *1T*-$TaS_2$ |
|---|---|---|---|---|---|---|---|
| | | CCDW | NCDW, $T_c$=310K | ICDW, $T_c$=370K | | | CCDW |
| coh. ph. | coh. ph | Raman | Raman | Raman | Raman | Raman | IR |
| | | | | | | 19 | |
| | | | | | 27 | | |
| | 42 (1.27) | | | | | | |
| | | | | | 48 | | 48 |
| | | | | | | | 54.5 |
| | | 56 | | | | | |
| | 59 (1.79) | | | | | | 58.5 |
| | | 62 | | | | | |
| | 63.8 (1.93) | | | | | | 63 |
| | | | 64 | | | 64 | |
| | | | | | | | 66.5 |
| | | 68 | | 68 | | | 68 |
| 68.9 (2.089) | 68.9 (2.089) | | | | | | |
| 71.5 (2.167) | 71.5 (2.167) | 71.5 | | | | 72 | 72 |
| 75.6 | 75.3 | 75 | | | 75 | | |
| | | 78 | | | | 78 | |
| | **78.9 (2.39)** | | | | | | |
| | | | | | | | 80 |
| **81.2(2.46)** | | | | | | | |
| | | 82 | | | | | |
| | | 84 | | | | | |
| | | 87.5 | | | | 88 | |
| | | | | | | | 89 |
| | | 92.5 | | | | | |
| | 96.35 | 95 | | | | 96 | |
| | 99.7 | 98.5 | | | | | 100 |
| | | 103 | | | | 103 | |
| 104.4 (3.165) | | | | | | | |
| | | 106 | | | | | 106 |
| | | 110 | | | | | |
| | | 114 | | | | | |
| | | 119 | | | | | |
| | | | | | | | 121 |
| | | 124 | | | | | |
| | | 127 | | | | | |
| 127.9 (3.875) | 127.9 (3.875) | | | | | | |
| | | | | | | 129 | 129 |
| | | | | | | | 134 |

TABLE I: Frequencies of the observed modes in the low frequency region for different polytypes of $TaS_2$ and their different phases[21–24]. Note that the laser power is significantly lower in time-resolved Pp spectroscopy than in Raman spectroscopy, which can explain the slightly higher frequencies of the coherent phonons compared to the Raman spectra. All energies are in wavenumbers ($cm^{-1}$). The numbers in brackets for the coherent phonons are in THz.

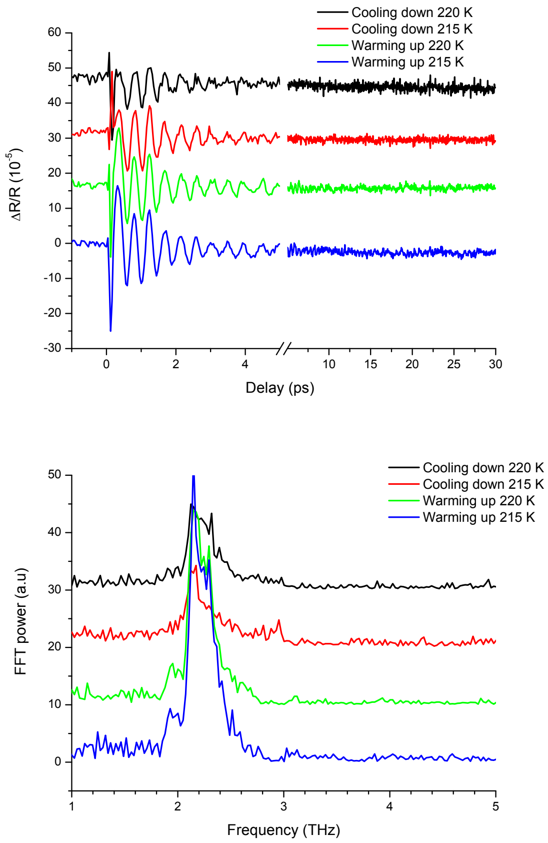


FIG. S6: Top: Transient reflectivity traces at different pump intensities measured by a pump-probe experiment in the NC state on cooling and the T state on warming. Note the absence of an additional exponentially decay component which could be attributed to single particle (SP) excitations. For comparison, the SP spectra are quite evident in the spectra shown in Fig. S5. Bottom: The corresponding power spectra show a relatively broad mode centered at 2.1 THz. Note that mode is not observed in either the H state spectra, or in the C state spectra.

---


[1] F. Zwick, et al. Spectral consequences of broken phase coherence in *1T*-$TaS_2$. Phys. Rev. Lett. **81**, 1058-1061 (1998).

[2] J. Demsar, L. Forro, H. Berger, & D. Mihailovic. Femtosecond snapshots of gap-forming charge-density-wave correlations in quasi-two-dimensional dichalcogenides *1T*-$TaS_2$ and *2H*-$TaSe_2$. Phys. Rev. B **66**, 041101 (2002).

[3] D. Mihailovic, et al. Femtosecond data storage, processing, and search using collective excita-

tions of a macroscopic quantum state. Appl. Phys. Lett. **80**, 871–873 (2002).

[4] T.Ishiguro and H.Sato, Electron microscopy of phase transformations in 1T-$TaS_2$. Phys. Rev.B **44**, 2046 (1991).

[5] D.Rideau, et al. X-ray scattering evidence for macroscopic strong pinning centers in the sliding CDW state of NbSe3, Europhys. Letters **56**, 289 (2001).

[6] P. Allen. Theory of thermal relaxation of electrons in metals. Phys. Rev. Lett. **59**, 1460-1463 (1987). V.V.Kabanov & A.S.Alexandrov, Electron relaxation in metals: Theory and exact analytical solutions. Phys Rev B **78**, 174514 (2008).

[7] J. Wilson, D. DiSalvo, F. & S.Mahajan, Charge-Density Waves and Superlattices in Metallic Layered Transition-Metal Dichalcogenides. Adv. Phys. **24**, 117-201 (1975).

[8] A. R. Beal, H. P. Hughes and W. Y. Liang, The reflectivity spectra of some group VA transition metal dichalcogenides, J. Phys. C: Solid State Phys. **8**, 4236 (1975).

[9] A. Suzuki, M. Koizumi, M. Doyama, Thermal evidences for successive CDW phase transitions in *1T*-$TaS_2$. Solid State Communications, **53**, 201 (1985).

[10] J. Bechtel, Heating of solid targets with laser pulses. J. Appl. Phys. **46**, 1585-1593 (1975).

[11] D. Nunez-Regueiro, J. Lopez-Castillo, & C. Ayache. Thermal Conductivity of *1T*-$TaS_2$ and *2H*-$TaSe_2$. Phys. Rev. Lett. **55**, 1931 (1985).

[12] R. Thomson, B. Burk, A. Zettl, and J, Clarke, *Phys Rev B* **49**, 16899–16916 (1994).

[13] For a review and refs. see P. Bak, Commensurate phases, incommensurate phases, and the devil's staircase, Rep. Prog. Phys., **45**, 597 (1982).

[14] J.C. Petersen et al., Clocking the Melting Transition of Charge and Lattice Order in 1T-$TaS_2$ with Ultrafast Extreme-Ultraviolet Angle-Resolved Photoemission Spectroscopy, Phys.Rev.Lett. **107,** 177402 (2011)

[15] J.K. Freericks1, H.R. Krishnamurthy, Yizhi Ge, A.Y. Liu & Th. Pruschke, Theoretical description of time-resolved pump/probe photoemission in TaS2: a single-band DFT+DMFT(NRG) study within the quasiequilibrium approximation, Phys. Status Solidi B **246**, 948954 (2009).

[16] Ju-Jin Kim, W. Yamaguchi, T. Hasegawa & K. Kitazawa, Observation of Mott Localization Gap Using Low Temperature Scanning Tunneling Spectroscopy in Commensurate 1T-TaS2, Phys. Rev. Lett. **73**, 2103 (1994).

[17] L. V. Gasparov and K. G. Brown, A.C. Wint, D.B. Tanner, H. Berger, G. Margaritondo, R. Gaal, and L. Forro, Phonon anomaly at the charge ordering transition in 1T-TaS2, Phys. Rev.

B **66**, 094301 (2002).

[18] J. Piprek, Semiconductor Optoelectronic devices (Academic Press, SanDiego, 2003).

[19] P.K.Basu, Theory of Optical Processes in Semiconductors: Bulk and Microstructures, Oxford University Press, 2003

[20] R.Yusupov et al., Coherent dynamics of macroscopic electronic order through a symmetry breaking transition, Nat Phys **6**, 681 (2010).

[21] J. R. Duffey and R. D. Kirby, Raman investigation of the charge-density-wave mixed-crystal system $1T$-$TaS_{2-x}Se_x$. J. Phys. Rev. B **23**, 1534 (1981); J.R. Duffey, R.D. Kirby, R.V. Coleman, Raman scattering from $1T$-$TaS_2$, Solid State Communications **20**, 617 (1976); Hirata, T. & Ohuchi, F. Temperature dependence of the Raman spectra of $1T$-$TaS_2$. Solid State Communications **117**, 361-364 (2001), S. Uchida, S. Sugai, Infrared and Raman studies on commensurate CDW states in transition metal dichalcogenides, Physica B+C **105**, 393-399 (1981).

[22] S. Sugai, K. Murase, S. Uchida, & S. Tanaka, Studies of Lattice-Dynamics in 2H-$TaS_2$ by Raman-Scattering. Solid State Communications **40**, 399-401 (1981).

[23] T. Nakashizu, T. Sekine, K. Uchinokura, & E. Matsuura, Raman-Study of Charge-Density-Wave Excitations in 4Hb-$TaS_2$. Phys Rev B **29**, 3090-3097 (1984); T. Nakashizu, T. Sekine, K. Uchinokura, and E. Matsuura, Raman Study of Charge-Density-Wave Phase Transitions in 4Hb-TaSe2. J. Phys. Soc. Jpn. **55**, 672-682 (1986).

[24] R. Kennedy and B. Clayman, Far-infrared studies of the commensurate charge-density wave of 1T-$TaS_2$. Phys. Rev. B**29**, 851-856 (1984); D. Karecki & B. Clayman, Far-infrared reflection spectra of 1T-$TaS_2$ and 1T-$TaSe_2$ in commensurate and incommensurate charge-density-wave states. Phys Rev B **19**, 6367-6371 (1979).
